# Supplementary material for: Accurate absolute and relative core-level binding energies from $GW$
Source: arXiv:1911.08428 ancillary file (2019-11-19)
Supplement: Supplementary file 1 [file supporting_information.pdf]

# Supporting information for:

## Accurate absolute and relative core-level binding energies from *GW*

Dorothea Golze,* Levi Keller, and Patrick Rinke

*Department of Applied Physics, Aalto University, Otakaari 1, FI-02150 Espoo, Finland*

E-mail: dorothea.golze@aalto.fi

## 1 Relative core-level binding energies

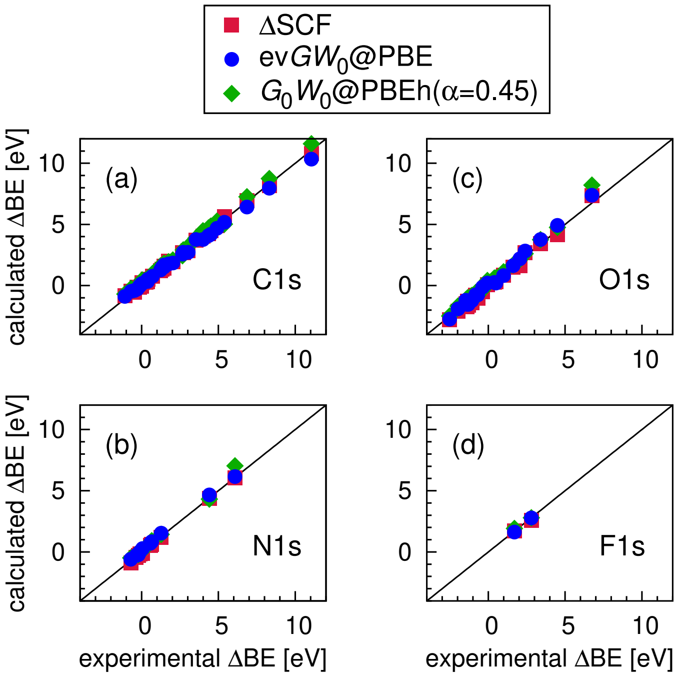


**Figure S1:** Relative C1s (a), N1s (b), O1s (c) and F1s (d) binding energies (ΔBEs) for the CORE65 benchmark set comparing calculated values at the ΔSCF, ev$GW_0$@PBE and $G_0W_0$@PBEh($\alpha$ = 0.45) level to experiment. Shift of the BE with respect to a reference molecule. $CH_4$, $NH_3$, $H_2O$ and $CH_3F$ have been used as reference molecules for C1s, N1s, O1s and F1s respectively.

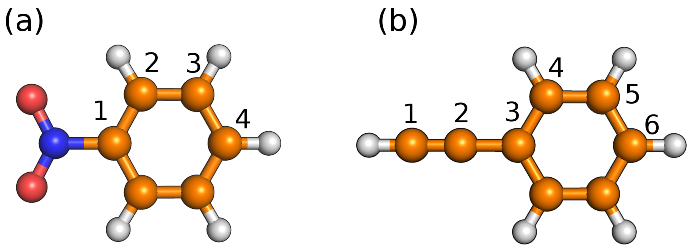


**Figure S2:** Labels for the carbon atoms for (a) nitrobenzene and (b) phenylacetylene. Color code: white, H; orange, C; blue, N; red, O.

## 2 CORE65 benchmark set

The computed and experimental core-level binding energies for the CORE65 benchmark set are given in Table S1. The labels for the carbon atoms of nitrobenzene and phenylacetylene are given in Figure S2. References in parentheses in Table S1 are the references from which the experimental value in the actual reference were retrieved, e.g., relative binding energy (BE) and BE of the reference compound. Relativistic corrections for ΔSCF are included self-consistently using ZORA and for *GW* we add the following relativistic corrections to the extrapolated results in Table S2 and S3: 0.118 eV for C1s, 0.236 eV for N1s, 0.424 eV for O1s and 0.708 eV for F1s.

Note that for $O_2$, a spin splitting of the O1s line occurs, i.e., the O1s peak is split in two peaks with the ratio 1:2. The weaker line is at higher and the stronger one at a lower binding energy.

**Table S1:** Core-level binding energies (BEs) as obtained from ΔSCF, ev$GW_0$@PBE and $G_0W_0$@PBEh($\alpha$=0.45) and deviation from experiment $\Delta_{\text{exp}}=\text{BE}_i^{\text{theory}} - \text{BE}_i^{\text{exp}}$. All values in eV. The ΔSCF values have been computed at the PBE0 level employing uncontracted def2-QZVP basis sets. For *GW*, BEs have been extrapolated to the complete basis set limit by performing a linear regression with respect to the inverse of the total number of basis functions using the cc-pV*n*Z basis set series ($n = 3 - 6$). Relativistic effects are taken into account for all three methods.

| | | | ΔSCF | | ev$GW_0$@PBE | | $G_0W_0$@PBEh | | | |
|---|---|---|---|---|---|---|---|---|---|---|
| name | formula | core level | BE | $\Delta_{\text{exp}}$ | BE | $\Delta_{\text{exp}}$ | BE | $\Delta_{\text{exp}}$ | Exp. | $\text{ref}_{\text{exp}}$ |
| methane | $CH_4$ | C1s | 290.46 | −0.39 | 290.62 | −0.22 | 290.80 | −0.04 | 290.84 | 1 |
| ethane | $C_2H_6$ | C1s | 290.33 | −0.39 | 290.59 | −0.12 | 290.80 | 0.09 | 290.71 | 1 |
| ethene | $C_2H_4$ | C1s | 290.43 | −0.40 | 290.74 | −0.08 | 290.87 | 0.05 | 290.82 | 1 |
| ethyne | $C_2H_2$ | C1s | 290.98 | −0.27 | 291.14 | −0.11 | 291.25 | 0.00 | 291.25 | 1 |
| carbon monoxide | CO | O1s | 542.21 | 0.11 | 542.16 | 0.06 | 541.69 | −0.41 | 542.1 | 2 |
| carbon monoxide | CO | C1s | 296.08 | −0.15 | 295.80 | −0.43 | 295.82 | −0.41 | 296.23 | 1 |
| carbon dioxide | $CO_2$ | O1s | 541.04 | −0.28 | 540.97 | −0.35 | 540.77 | −0.55 | 541.32 | 3 |
| carbon dioxide | $CO_2$ | C1s | 297.42 | −0.28 | 297.04 | −0.66 | 298.06 | 0.36 | 297.70 | 1 |
| tetrafluoromethane | $CF_4$ | F1s | 695.06 | −0.14 | 694.77 | −0.43 | 694.29 | −0.91 | 695.2 | 4 |
| tetrafluoromethane | $CF_4$ | C1s | 301.26 | −0.64 | 300.96 | −0.93 | 302.39 | 0.49 | 301.90 | 1 |
| fluoromethane | $CH_3F$ | F1s | 692.49 | 0.09 | 691.99 | −0.41 | 691.50 | −0.90 | 692.4 | 5 |
| fluoromethane | $CH_3F$ | C1s | 293.16 | −0.40 | 293.35 | −0.21 | 293.71 | 0.15 | 293.56 | 1 |
| trifluoromethane | $CHF_3$ | F1s | 694.23 | 0.13 | 693.62 | −0.48 | 693.41 | −0.69 | 694.1 | 5 |
| trifluoromethane | $CHF_3$ | C1s | 298.62 | −0.54 | 298.58 | −0.58 | 299.55 | 0.39 | 299.16 | 1 |
| methanol | $CH_3OH$ | O1s | 538.73 | −0.15 | 538.60 | −0.28 | 538.51 | −0.37 | 538.88 | 6 (7,8) |
| methanol | $CH_3OH$ | C1s | 292.06 | −0.24 | 292.31 | 0.01 | 292.62 | 0.32 | 292.3 | 2,6 |
| formaldehyde | $CH_2O$ | O1s | 539.04 | −0.29 | 539.22 | −0.11 | 538.72 | −0.61 | 539.33 | 6 (7,8) |
| formaldehyde | $CH_2O$ | C1s | 294.16 | −0.22 | 294.39 | 0.01 | 294.68 | 0.30 | 294.38 | 6 |
| dimethyl ether | $CH_3OCH_3$ | O1s | 538.25 | −0.11 | 538.11 | −0.25 | 538.07 | −0.29 | 538.36 | 6 (7,8) |
| dimethyl ether | $CH_3OCH_3$ | C1s | 291.81 | −0.36 | 292.10 | −0.07 | 292.37 | 0.20 | 292.17 | 9 |
| formic acid | HCOOH | O1s (OH) | 540.39 | −0.30 | 540.16 | −0.53 | 540.20 | −0.49 | 540.69 | 10 |
| formic acid | HCOOH | O1s (C=O) | 538.51 | −0.51 | 538.59 | −0.43 | 538.29 | −0.73 | 539.02 | 10 |
| formic acid | HCOOH | C1s | 295.37 | −0.38 | 295.30 | −0.45 | 296.06 | 0.31 | 295.75 | 10 |

**Table S1:** Continued

| | | | ΔSCF | | ev$GW_0$@PBE | | $G_0W_0$@PBEh | | | |
|---|---|---|---|---|---|---|---|---|---|---|
| name | formula | core level | $\Delta_{exp}$ | BE | $\Delta_{exp}$ | BE | $\Delta_{exp}$ | Exp. | $ref_{exp}$ | |
| acetone | $(CH_3)_2CO$ | O1s | 537.43 | −0.30 | 537.44 | −0.29 | 537.40 | −0.33 | 537.73 | 6 (7,8) |
| acetone | $(CH_3)_2CO$ | C1s (C=O) | 293.31 | −0.57 | 293.35 | −0.53 | 294.00 | 0.12 | 293.88 | 6 |
| acetone | $(CH_3)_2CO$ | C1s ($CH_3$) | 290.77 | −0.46 | 290.96 | −0.27 | 291.35 | 0.12 | 291.23 | 6 |
| methyl formate | $HCO_2CH_3$ | O1s ($OCH_3$) | 539.60 | −0.04 | 539.56 | −0.08 | 539.48 | −0.16 | 539.64 | 6 (7,8) |
| methyl formate | $HCO_2CH_3$ | O1s (C=O) | 538.03 | −0.21 | 538.14 | −0.10 | 537.93 | −0.31 | 538.24 | 6 (7,8) |
| acetic acid | $CH_3COOH$ | O1s (OH) | 539.82 | −0.28 | 539.61 | −0.49 | 539.69 | −0.41 | 540.10 | 10 |
| acetic acid | $CH_3COOH$ | O1s (C=O) | 537.80 | −0.51 | 537.81 | −0.50 | 537.66 | −0.65 | 538.31 | 10 |
| acetic acid | $CH_3COOH$ | C1s (COOH) | 294.93 | −0.42 | 294.82 | −0.53 | 295.66 | 0.31 | 295.35 | 10 |
| acetic acid | $CH_3COOH$ | C1s ($CH_3$) | 291.21 | −0.34 | 291.39 | −0.16 | 291.78 | 0.23 | 291.55 | 10 |
| water | $H_2O$ | O1s | 539.53 | −0.17 | 539.34 | −0.36 | 539.08 | −0.62 | 539.7 | 8 |
| ozone | $O_3$ | O1s middle | 546.89 | 0.45 | 546.73 | 0.29 | 547.29 | 0.85 | 546.44 | 11 |
| ozone | $O_3$ | O1s terminal | 541.17 | −0.58 | 541.53 | −0.22 | 541.20 | −0.55 | 541.75 | 11 |
| oxygen | $O_2$ | O1s weaker | 543.67 | −0.53 | 544.27 | 0.07 | 543.83 | −0.37 | 544.2 | 8 |
| oxygen | $O_2$ | O1s stronger | 542.95 | −0.15 | 543.10 | 0.00 | 542.83 | −0.27 | 543.1 | 8 |
| nitrogen | $N_2$ | N1s | 409.65 | −0.28 | 409.75 | −0.18 | 409.63 | −0.30 | 409.93 | 3 |
| ammonia | $NH_3$ | N1s | 405.27 | −0.25 | 405.09 | −0.43 | 405.32 | −0.20 | 405.52 | 6 (3,7) |
| hydrogen cyanide | HCN | N1s | 406.48 | −0.32 | 406.62 | −0.18 | 406.75 | −0.05 | 406.8 | 6 (3,12) |
| hydrogen cyanide | HCN | C1s | 293.14 | −0.36 | 293.19 | −0.31 | 293.24 | −0.26 | 293.5 | 6 |
| acetonitrile | $CH_3CN$ | N1s | 405.15 | −0.43 | 405.37 | −0.21 | 405.43 | −0.15 | 405.58 | 13 |
| acetonitrile | $CH_3CN$ | C1s ($CH_3$) | 292.39 | −0.49 | 292.47 | −0.41 | 292.89 | 0.01 | 292.88 | 13 |
| acetonitrile | $CH_3CN$ | C1s (CN) | 292.43 | −0.17 | 292.40 | −0.20 | 292.74 | 0.14 | 292.60 | 13 |
| glycine | $C_2H_5NO_2$ | O1s (OH) | 539.85 | −0.35 | 539.55 | −0.65 | 539.70 | −0.50 | 540.2 | 14 |
| glycine | $C_2H_5NO_2$ | O1s (C=O) | 537.90 | −0.50 | 537.81 | −0.59 | 537.81 | −0.59 | 538.4 | 14 |
| glycine | $C_2H_5NO_2$ | N1s | 405.14 | −0.26 | 405.09 | −0.31 | 405.43 | 0.03 | 405.4 | 14 |
| glycine | $C_2H_5NO_2$ | C1s (COOH) | 294.71 | −0.49 | 294.70 | −0.50 | 295.52 | 0.32 | 295.2 | 14 |
| glycine | $C_2H_5NO_2$ | C1s ($CH_2$) | 291.88 | −0.42 | 292.14 | −0.16 | 292.55 | 0.25 | 292.3 | 14 |
| pyridine | $C_5H_5N$ | N1s | 404.35 | −0.47 | 404.50 | −0.32 | 404.83 | 0.01 | 404.82 | 15 |
| pyrrole | $C_4H_4NH$ | N1s | 405.90 | −0.28 | 405.93 | −0.25 | 406.23 | 0.05 | 406.18 | 15 |
| aniline | $C_6H_5NH_2$ | N1s | 405.00 | −0.31 | 404.86 | −0.45 | 405.11 | −0.20 | 405.31 | 15 |
| urea | $CO(NH_2)_2$ | O1s | 536.73 | −0.46 | 536.60 | −0.59 | 536.59 | −0.60 | 537.19 | 6 |
| urea | $CO(NH_2)_2$ | N1s | 405.79 | −0.30 | 405.80 | −0.29 | 406.08 | −0.01 | 406.09 | 6 |
| urea | $CO(NH_2)_2$ | C1s | 294.51 | −0.33 | 294.39 | −0.45 | 295.27 | 0.43 | 294.84 | 6 |
| methylamine | $CH_3NH_2$ | N1s | 404.84 | −0.33 | 404.82 | −0.35 | 405.14 | −0.03 | 405.17 | 6 (3,7) |
| nitrobenzene | $C_6H_5NO_2$ | O1s | 538.10 | −0.53 | 538.11 | −0.52 | 538.27 | −0.36 | 538.63 | 6 |
| nitrobenzene | $C_6H_5NO_2$ | N1s | 411.32 | −0.28 | 411.25 | −0.35 | 412.36 | 0.76 | 411.6 | 2 |
| nitrobenzene | $C_6H_5NO_2$ | C1s (C1) | 291.67 | −0.41 | 291.90 | −0.18 | 292.42 | 0.34 | 292.08 | 6 |
| nitrobenzene | $C_6H_5NO_2$ | C1s (C2-4) | 290.71 | −0.42 | 290.96 | −0.17 | 291.29 | 0.16 | 291.13 | 6 |
| benzene | $C_6H_6$ | C1s | 289.93 | −0.45 | 290.23 | −0.15 | 290.47 | 0.09 | 290.38 | 16 |
| phenylacetylene | $C_8H_6$ | C1s (C3) | 290.71 | −0.17 | 290.79 | −0.09 | 291.27 | 0.39 | 290.88 | 17 |
| phenylacetylene | $C_8H_6$ | C1s (C2) | 290.31 | −0.24 | 290.34 | −0.21 | 290.74 | 0.19 | 290.55 | 17 |
| phenylacetylene | $C_8H_6$ | C1s (C4-6) | 289.98 | −0.18 | 290.15 | −0.01 | 290.56 | 0.40 | 290.16 | 17 |
| phenylacetylene | $C_8H_6$ | C1s (C1) | 289.60 | −0.15 | 289.74 | −0.01 | 290.11 | 0.36 | 289.75 | 17 |

# 3 ev$GW_0$ results without relativistic correction

For the basis set extrapolation we observe a clear trend. The core-level BEs increase with increasing number of basis functions. The largest basis sets, cc-pV5Z and cc-pV6Z, have a spectrum of virtual states up to several thousand eV. Charge neutral excitations $\Omega_s$ to these high energy states lead to a few additional small poles in the core region. This is an artifact of finite basis sets and the spectrum in the unoccupied should become continuous in the infinite basis set limit. However, these artifact can disturb in some cases the extrapolation and we therefore exclude

for some excitations the cc-pV5Z and cc-pV6Z data points from the extrapolation. Furthermore, the computational cost for ev$GW_0$ with the cc-pV6Z is for the largest molecules very demanding since we include all occupied states explicitly in the calculation. In two cases, we used thus only $n = 3 - 5$ for the extrapolation.

**Table S2:** Non-relativistic core-level binding from ev$GW_0$@PBE using the cc-pV$n$Z basis set series with $n = 3-6$. Extrapolated values ($\infty$), standard error (SE) and correlation coefficient $R^2$. The last column gives the basis sets used for the extrapolation; for most cases all data points ($n = 3 - 6$) are included. All values in eV.

| | | | | ev$GW_0$@PBE | | | | | | | |
|---|---|---|---|---|---|---|---|---|---|---|---|
| CAS | name | formula | core level | $n = 3$ | $n = 4$ | $n = 5$ | $n = 6$ | $\infty$ | SE | $R^2$ | $n$ used |
| 74-82-8 | methane | $CH_4$ | C1s | 289.83 | 290.08 | 290.21 | 290.51 | 290.51 | 0.12 | 0.86 | 3-6 |
| 74-84-0 | ethane | $C_2H_6$ | C1s | 289.73 | 290.04 | 290.19 | 290.43 | 290.47 | 0.08 | 0.94 | 3-6 |
| 74-85-1 | ethene | $C_2H_4$ | C1s | 290.02 | 290.29 | 290.38 | 290.58 | 290.62 | 0.07 | 0.94 | 3-6 |
| 74-86-2 | ethyne | $C_2H_2$ | C1s | 290.51 | 290.74 | 290.78 | 291.00 | 291.02 | 0.07 | 0.90 | 3-6 |
| 630-08-0 | carbon monoxide | CO | O1s | 541.27 | 541.45 | 541.58 | 541.65 | 541.74 | 0.02 | 0.99 | 3-6 |
| 630-08-0 | carbon monoxide | CO | C1s | 295.10 | 295.39 | 295.48 | 295.55 | 295.68 | 0.02 | 0.99 | 3-6 |
| 124-38-9 | carbon dioxide | $CO_2$ | O1s | 540.03 | 540.27 | 540.24 | 540.37 | 540.55 | | | 3,4 |
| 124-38-9 | carbon dioxide | $CO_2$ | C1s | 296.14 | 296.48 | 296.59 | 296.82 | 296.93 | 0.07 | 0.96 | 3-6 |
| 75-73-0 | tetrafluoromethane | $CF_4$ | F1s | 693.36 | 693.50 | 693.58 | 693.74 | 694.06 | | | 5,6 |
| 75-73-0 | tetrafluoromethane | $CF_4$ | C1s | 299.89 | 300.32 | 300.46 | 300.70 | 300.85 | 0.07 | 0.98 | 3-6 |
| 593-53-3 | fluoromethane | $CH_3F$ | F1s | 690.98 | 691.16 | 691.09 | 691.21 | 691.28 | 0.03 | 0.97 | 3,4,6 |
| 593-53-3 | fluoromethane | $CH_3F$ | C1s | 292.45 | 292.79 | 292.95 | 293.14 | 293.23 | 0.06 | 0.97 | 3-6 |
| 75-46-7 | trifluoromethane | $CHF_3$ | F1s | 692.59 | 692.73 | 692.75 | 692.89 | 692.91 | 0.05 | 0.88 | 3-6 |
| 75-46-7 | trifluoromethane | $CHF_3$ | C1s | 297.51 | 297.94 | 298.09 | 298.33 | 298.46 | 0.07 | 0.97 | 3-6 |
| 67-56-1 | methanol | $CH_3OH$ | O1s | 537.84 | 538.00 | 537.97 | 538.11 | 538.17 | 0.01 | 1.00 | 3,4,6 |
| 67-56-1 | methanol | $CH_3OH$ | C1s | 291.41 | 291.74 | 291.85 | 292.16 | 292.19 | 0.11 | 0.90 | 3-6 |
| 50-00-0 | formaldehyde | $CH_2O$ | O1s | 538.14 | 538.46 | 538.46 | 538.56 | 538.80 | | | 3,4 |
| 50-00-0 | formaldehyde | $CH_2O$ | C1s | 293.48 | 293.89 | 293.98 | 294.16 | 294.27 | 0.05 | 0.98 | 3-6 |
| 115-10-6 | dimethyl ether | $CH_3OCH_3$ | O1s | 537.40 | 537.51 | 537.55 | 537.69 | 537.69 | 0.05 | 0.85 | 3-6 |
| 115-10-6 | dimethyl ether | $CH_3OCH_3$ | C1s | 291.22 | 291.53 | 291.67 | 291.94 | 291.98 | 0.09 | 0.93 | 3-6 |
| 64-18-6 | formic acid | HCOOH | O1s (OH) | 539.37 | 539.56 | 539.56 | 539.70 | 539.73 | 0.05 | 0.89 | 3-6 |
| 64-18-6 | formic acid | HCOOH | O1s (C=O) | 537.47 | 537.80 | 537.78 | 537.89 | 538.16 | | | 3,4 |
| 64-18-6 | formic acid | HCOOH | C1s | 294.34 | 294.78 | 294.84 | 295.08 | 295.19 | 0.07 | 0.96 | 3-6 |
| 67-64-1 | acetone | $(CH_3)_2CO$ | O1s | 536.56 | 536.79 | 536.79 | 536.93 | 537.01 | 0.01 | 1.00 | 3,4,6 |
| 67-64-1 | acetone | $(CH_3)_2CO$ | C1s (C=O) | 292.56 | 292.85 | 292.96 | 293.18 | 293.23 | 0.07 | 0.95 | 3-6 |
| 67-64-1 | acetone | $(CH_3)_2CO$ | C1s ($CH_3$) | 290.12 | 290.41 | 290.55 | 290.79 | 290.84 | 0.08 | 0.93 | 3-6 |
| 107-31-3 | methyl formate | $HCO_2CH_3$ | O1s ($OCH_3$) | 538.65 | 538.84 | 538.91 | 539.12 | 539.13 | 0.08 | 0.88 | 3-6 |
| 107-31-3 | methyl formate | $HCO_2CH_3$ | O1s (C=O) | 537.01 | 537.35 | 537.33 | 537.43 | 537.72 | | | 3,4 |
| 64-19-7 | acetic acid | $CH_3COOH$ | O1s (OH) | 538.79 | 538.97 | 538.96 | 539.11 | 539.18 | 0.01 | 1.00 | 3,4,6 |
| 64-19-7 | acetic acid | $CH_3COOH$ | O1s (C=O) | 536.78 | 537.07 | 537.06 | 537.19 | 537.39 | | | 3,4 |
| 64-19-7 | acetic acid | $CH_3COOH$ | C1s (COOH) | 293.97 | 294.26 | 294.39 | 294.67 | 294.71 | 0.10 | 0.91 | 3-6 |
| 64-19-7 | acetic acid | $CH_3COOH$ | C1s ($CH_3$) | 290.55 | 290.79 | 290.95 | 291.26 | 291.27 | 0.13 | 0.87 | 3-6 |
| 7732-18-5 | water | $H_2O$ | O1s | 538.59 | 538.75 | 538.68 | 538.78 | 538.92 | | | 3,4 |
| 10028-15-6 | ozone | $O_3$ | O1s middle | 545.89 | 546.08 | 546.17 | 546.31 | 546.31 | 0.00 | 1.00 | 3-5 |
| 10028-15-6 | ozone | $O_3$ | O1s terminal | 540.56 | 540.81 | 540.79 | 540.86 | 541.10 | | | 3,4 |
| 7782-44-7 | oxygen | $O_2$ | O1s weaker | 543.23 | 543.51 | 543.46 | | 543.85 | | | 3,4 |
| 7782-44-7 | oxygen | $O_2$ | O1s stronger | 541.98 | 542.30 | 542.38 | | 542.68 | | | 3,4 |
| 7727-37-9 | nitrogen | $N_2$ | N1s | 408.70 | 409.08 | 409.20 | 409.37 | 409.52 | 0.04 | 0.99 | 3-6 |
| 7664-41-7 | ammonia | $NH_3$ | N1s | 404.63 | 404.73 | 404.80 | 405.06 | 404.85 | 0.01 | 0.99 | 3-5 |
| 74-90-8 | hydrogen cyanide | HCN | N1s | 405.75 | 406.12 | 406.09 | 406.31 | 406.39 | 0.09 | 0.90 | 3-6 |
| 74-90-8 | hydrogen cyanide | HCN | C1s | 292.50 | 292.74 | 292.82 | 293.03 | 293.07 | 0.07 | 0.93 | 3-6 |
| 75-05-8 | acetonitrile | $CH_3CN$ | N1s | 404.49 | 404.83 | 404.81 | 405.09 | 405.13 | 0.10 | 0.88 | 3-6 |
| 75-05-8 | acetonitrile | $CH_3CN$ | C1s ($CH_3$) | 291.66 | 291.95 | 292.05 | 292.31 | 292.36 | 0.09 | 0.92 | 3-6 |
| 75-05-8 | acetonitrile | $CH_3CN$ | C1s (CN) | 291.69 | 291.94 | 292.03 | 292.24 | 292.28 | 0.07 | 0.93 | 3-6 |
| 56-40-6 | glycine | $C_2H_5NO_2$ | O1s (OH) | 538.79 | 538.95 | 538.99 | 539.23 | 539.12 | | | 3,4 |

**Table S2:** Continued

| | | | | $evGW_0$@PBE | | | | | | | |
|---|---|---|---|---|---|---|---|---|---|---|---|
| CAS | name | formula | core level | $n=3$ | $n=4$ | $n=5$ | $n=6$ | ∞ | SE | $R^2$ | $n$ used |
| 56-40-6 | glycine | $C_2H_5NO_2$ | O1s (C=O) | 536.87 | 537.13 | 537.15 | 537.28 | 537.39 | 0.01 | 1.00 | 3,4,6 |
| 56-40-6 | glycine | $C_2H_5NO_2$ | N1s | 404.50 | 404.65 | 404.76 | 405.00 | 404.86 | 0.04 | 0.98 | 3-5 |
| 56-40-6 | glycine | $C_2H_5NO_2$ | C1s (COOH) | 293.71 | 294.11 | 294.25 | 294.47 | 294.58 | 0.06 | 0.97 | 3-6 |
| 56-40-6 | glycine | $C_2H_5NO_2$ | C1s ($CH_2$) | 291.12 | 291.52 | 291.68 | 291.92 | 292.02 | 0.07 | 0.97 | 3-6 |
| 110-86-1 | pyridine | $C_5H_5N$ | N1s | 403.69 | 403.91 | 404.02 | 404.22 | 404.26 | 0.07 | 0.92 | 3-6 |
| 109-97-7 | pyrrole | $C_4H_4NH$ | N1s | 404.98 | 405.28 | 405.43 | 405.62 | 405.70 | 0.06 | 0.97 | 3-6 |
| 62-53-3 | aniline | $C_6H_5NH_2$ | N1s | 404.04 | 404.34 | 404.44 | | 404.63 | 0.02 | 1.00 | 3-5 |
| 57-13-6 | urea | $CO(NH_2)_2$ | O1s | 535.64 | 535.90 | 536.04 | 536.05 | 536.17 | 0.02 | 0.99 | 3-6 |
| 57-13-6 | urea | $CO(NH_2)_2$ | N1s | 404.95 | 405.15 | 405.30 | 405.54 | 405.56 | 0.10 | 0.88 | 3-6 |
| 57-13-6 | urea | $CO(NH_2)_2$ | C1s | 293.45 | 293.76 | 293.96 | 294.20 | 294.27 | 0.09 | 0.95 | 3-6 |
| 74-89-5 | methylamine | $CH_3NH_2$ | N1s | 404.26 | 404.42 | 404.45 | 404.73 | 404.58 | | | 3,4 |
| 98-95-3 | nitrobenzene | $C_6H_5NO_2$ | O1s | 537.36 | 537.49 | 537.61 | 537.61 | 537.69 | 0.03 | 0.96 | 3-6 |
| 98-95-3 | nitrobenzene | $C_6H_5NO_2$ | N1s | 410.23 | 410.52 | 410.68 | 410.96 | 411.01 | 0.10 | 0.92 | 3-6 |
| 98-95-3 | nitrobenzene | $C_6H_5NO_2$ | C1s (C1) | 290.99 | 291.29 | 291.43 | 291.74 | 291.79 | 0.11 | 0.91 | 3-6 |
| 98-95-3 | nitrobenzene | $C_6H_5NO_2$ | C1s (C2-4) | 290.16 | 290.37 | 290.53 | 290.83 | 290.85 | 0.13 | 0.86 | 3-6 |
| 71-43-2 | benzene | $C_6H_6$ | C1s | 289.41 | 289.71 | 289.84 | 290.03 | 290.11 | 0.06 | 0.96 | 3-6 |
| 536-74-3 | phenylacetylene | $C_8H_6$ | C1s (C3) | 290.04 | 290.36 | 290.47 | | 290.67 | 0.03 | 1.00 | 3-5 |
| 536-74-3 | phenylacetylene | $C_8H_6$ | C1s (C2) | 289.60 | 289.92 | 290.02 | | 290.22 | 0.04 | 0.99 | 3-5 |
| 536-74-3 | phenylacetylene | $C_8H_6$ | C1s (C4-6) | 289.41 | 289.72 | 289.84 | | 290.03 | 0.01 | 1.00 | 3-5 |
| 536-74-3 | phenylacetylene | $C_8H_6$ | C1s (C1) | 289.13 | 289.39 | 289.46 | | 289.62 | 0.04 | 0.99 | 3-5 |

# 4 $G_0W_0$ results without relativistic correction

**Table S3:** Non-relativistic core-level binding from $G_0W_0$@PBEh($\alpha = 0.45$) using the cc-pV$n$Z basis set series with $n = 3-6$. Extrapolated values (∞), standard error (SE) and correlation coefficient $R^2$. The last column gives the basis sets used for the extrapolation; for most cases all data points ($n = 3-6$) are included. All values in eV.

| | | | | $G_0W_0$@PBEh($\alpha = 0.45$) | | | | | | | |
|---|---|---|---|---|---|---|---|---|---|---|---|
| CAS | name | formula | core level | $n=3$ | $n=4$ | $n=5$ | $n=6$ | ∞ | SE | $R^2$ | $n$ used |
| 74-82-8 | methane | $CH_4$ | C1s | 290.20 | 290.40 | 290.52 | 290.64 | 290.68 | 0.04 | 0.96 | 3-6 |
| 74-84-0 | ethane | $C_2H_6$ | C1s | 290.18 | 290.39 | 290.38 | 290.62 | 290.69 | 0.05 | 0.98 | 3,4,6 |
| 74-85-1 | ethene | $C_2H_4$ | C1s | 290.35 | 290.54 | 290.62 | 290.70 | 290.76 | 0.02 | 0.99 | 3-6 |
| 74-86-2 | ethyne | $C_2H_2$ | C1s | 290.80 | 290.89 | 290.85 | 291.10 | 291.13 | 0.09 | 0.87 | 3,4,6 |
| 630-08-0 | carbon monoxide | CO | O1s | 541.15 | 541.18 | 541.23 | 541.25 | 541.26 | 0.01 | 0.93 | 3-6 |
| 630-08-0 | carbon monoxide | CO | C1s | 295.48 | 295.58 | 295.58 | 295.56 | 295.70 | | | 3,4 |
| 124-38-9 | carbon dioxide | $CO_2$ | O1s | 540.22 | 540.28 | 540.30 | 540.42 | 540.34 | 0.02 | 0.97 | 3,4,5 |
| 124-38-9 | carbon dioxide | $CO_2$ | C1s | 297.39 | 297.61 | 297.62 | 297.84 | 297.94 | 0.04 | 0.99 | 3,4,6 |
| 75-73-0 | tetrafluoromethane | $CF_4$ | F1s | 693.65 | 693.61 | 693.55 | 693.60 | 693.59 | 0.01 | 0.93 | 3,4,6 |
| 75-73-0 | tetrafluoromethane | $CF_4$ | C1s | 301.60 | 301.91 | 301.98 | 302.17 | 302.27 | 0.06 | 0.96 | 3-6 |
| 593-53-3 | fluoromethane | $CH_3F$ | F1s | 690.81 | 690.78 | 690.70 | 690.79 | 690.79 | | | 3,6 |
| 593-53-3 | fluoromethane | $CH_3F$ | C1s | 293.00 | 293.27 | 293.34 | 293.55 | 293.59 | 0.07 | 0.93 | 3-6 |
| 75-46-7 | trifluoromethane | $CHF_3$ | F1s | 692.70 | 692.67 | 692.62 | 692.70 | 692.70 | | | 3,6 |
| 75-46-7 | trifluoromethane | $CHF_3$ | C1s | 298.76 | 299.08 | 299.14 | 299.35 | 299.43 | 0.07 | 0.95 | 3-6 |
| 67-56-1 | methanol | $CH_3OH$ | O1s | 537.93 | 537.98 | 537.94 | 538.07 | 538.08 | 0.02 | 0.95 | 3,4,6 |
| 67-56-1 | methanol | $CH_3OH$ | C1s | 291.91 | 292.16 | 292.27 | 292.45 | 292.50 | 0.06 | 0.95 | 3-6 |
| 50-00-0 | formaldehyde | $CH_2O$ | O1s | 538.15 | 538.21 | 538.15 | 538.28 | 538.30 | 0.02 | 0.97 | 3,4,6 |
| 50-00-0 | formaldehyde | $CH_2O$ | C1s | 294.03 | 294.27 | 294.36 | 294.49 | 294.56 | 0.03 | 0.98 | 3-6 |

**Table S3:** Continued

| CAS | name | formula | core level | $G_0W_0$@PBEh($\alpha$ = 0.45) | | | | | SE | $R^2$ | $n$ used |
|---|---|---|---|---|---|---|---|---|---|---|---|
| | | | | $n$ = 3 | $n$ = 4 | $n$ = 5 | $n$ = 6 | ∞ | | | |
| 115-10-6 | dimethyl ether | $CH_3OCH_3$ | O1s | 537.56 | 537.61 | 537.62 | 537.75 | 537.65 | 0.00 | 1.00 | 3,4,5 |
| 115-10-6 | dimethyl ether | $CH_3OCH_3$ | C1s | 291.72 | 291.96 | 292.06 | 292.21 | 292.26 | 0.04 | 0.96 | 3-6 |
| 64-18-6 | formic acid | HCOOH | O1s (OH) | 539.56 | 539.63 | 539.70 | 539.76 | 539.78 | 0.03 | 0.93 | 3-6 |
| 64-18-6 | formic acid | HCOOH | O1s (C=O) | 537.68 | 537.75 | 537.81 | 537.83 | 537.86 | 0.01 | 0.99 | 3-6 |
| 64-18-6 | formic acid | HCOOH | C1s | 295.36 | 295.62 | 295.74 | 295.86 | 295.95 | 0.03 | 0.99 | 3-6 |
| 67-64-1 | acetone | $(CH_3)_2CO$ | O1s | 536.76 | 536.82 | 536.92 | 536.94 | 536.97 | 0.03 | 0.93 | 3-6 |
| 67-64-1 | acetone | $(CH_3)_2CO$ | C1s (C=O) | 293.41 | 293.59 | 293.73 | 293.83 | 293.88 | 0.04 | 0.97 | 3-6 |
| 67-64-1 | acetone | $(CH_3)_2CO$ | C1s ($CH_3$) | 290.69 | 290.91 | 291.02 | 291.18 | 291.23 | 0.05 | 0.96 | 3-6 |
| 107-31-3 | methyl formate | $HCO_2CH_3$ | O1s ($OCH_3$) | 538.95 | 539.01 | 539.02 | 539.15 | 539.06 | 0.01 | 0.98 | 3,4,5 |
| 107-31-3 | methyl formate | $HCO_2CH_3$ | O1s (C=O) | 537.30 | 537.37 | 537.43 | 537.48 | 537.50 | 0.02 | 0.95 | 3-6 |
| 64-19-7 | acetic acid | $CH_3COOH$ | O1s (OH) | 539.05 | 539.12 | 539.18 | 539.25 | 539.27 | 0.03 | 0.90 | 3-6 |
| 64-19-7 | acetic acid | $CH_3COOH$ | O1s (C=O) | 537.04 | 537.12 | 537.16 | 537.21 | 537.23 | 0.02 | 0.94 | 3-6 |
| 64-19-7 | acetic acid | $CH_3COOH$ | C1s (COOH) | 295.03 | 295.26 | 295.31 | 295.50 | 295.54 | 0.06 | 0.92 | 3-6 |
| 64-19-7 | acetic acid | $CH_3COOH$ | C1s ($CH_3$) | 291.10 | 291.34 | 291.43 | 291.61 | 291.66 | 0.06 | 0.95 | 3-6 |
| 7732-18-5 | water | $H_2O$ | O1s | 538.55 | 538.60 | 538.50 | 538.49 | 538.65 | | | 3,4 |
| 10028-15-6 | ozone | $O_3$ | O1s middle | 546.73 | 546.79 | 546.82 | 546.91 | 546.87 | 0.00 | 1.00 | 3,4,5 |
| 10028-15-6 | ozone | $O_3$ | O1s terminal | 540.72 | 540.74 | 540.76 | 540.83 | 540.77 | 0.01 | 0.95 | 3,4,5 |
| 7782-44-7 | oxygen | $O_2$ | O1s weaker | 543.37 | 543.36 | 543.33 | 543.40 | 543.41 | | | 3,6 |
| 7782-44-7 | oxygen | $O_2$ | O1s stronger | 542.33 | 542.32 | 542.32 | 542.39 | 542.41 | | | 3,6 |
| 7727-37-9 | nitrogen | $N_2$ | N1s | 409.08 | 409.21 | 409.28 | 409.35 | 409.40 | 0.02 | 0.98 | 3-6 |
| 7664-41-7 | ammonia | $NH_3$ | N1s | 404.73 | 404.91 | 404.70 | 405.02 | 405.08 | 0.00 | 1.00 | 3,4,6 |
| 74-90-8 | hydrogen cyanide | HCN | N1s | 405.96 | 406.17 | 406.13 | 406.43 | 406.52 | 0.06 | 0.97 | 3,4,6 |
| 74-90-8 | hydrogen cyanide | HCN | C1s | 292.80 | 292.94 | 293.00 | 293.08 | 293.12 | 0.02 | 0.97 | 3-6 |
| 75-05-8 | acetonitrile | $CH_3CN$ | N1s | 404.85 | 405.00 | 404.94 | 405.13 | 405.19 | 0.01 | 1.00 | 3,4,6 |
| 75-05-8 | acetonitrile | $CH_3CN$ | C1s ($CH_3$) | 292.22 | 292.45 | 292.57 | 292.72 | 292.77 | 0.05 | 0.96 | 3-6 |
| 75-05-8 | acetonitrile | $CH_3CN$ | C1s (CN) | 292.19 | 292.35 | 292.33 | 292.56 | 292.63 | 0.05 | 0.97 | 3,4,6 |
| 56-40-6 | glycine | $C_2H_5NO_2$ | O1s (OH) | 539.12 | 539.20 | 539.22 | 539.33 | 539.27 | 0.00 | 1.00 | 3,4,5 |
| 56-40-6 | glycine | $C_2H_5NO_2$ | O1s (C=O) | 537.16 | 537.25 | 537.33 | 537.35 | 537.39 | 0.02 | 0.97 | 3-6 |
| 56-40-6 | glycine | $C_2H_5NO_2$ | N1s | 404.80 | 404.96 | 405.02 | 405.17 | 405.19 | 0.05 | 0.92 | 3-6 |
| 56-40-6 | glycine | $C_2H_5NO_2$ | C1s (COOH) | 294.83 | 295.10 | 295.18 | 295.33 | 295.40 | 0.04 | 0.97 | 3-6 |
| 56-40-6 | glycine | $C_2H_5NO_2$ | C1s ($CH_2$) | 291.86 | 292.10 | 292.22 | 292.37 | 292.43 | 0.05 | 0.96 | 3-6 |
| 110-86-1 | pyridine | $C_5H_5N$ | N1s | 404.15 | 404.33 | 404.45 | 404.53 | 404.60 | 0.03 | 0.98 | 3-6 |
| 109-97-7 | pyrrole | $C_4H_4NH$ | N1s | 405.65 | 405.75 | 405.75 | 405.95 | 406.00 | 0.07 | 0.92 | 3,4,6 |
| 62-53-3 | aniline | $C_6H_5NH_2$ | N1s | 404.43 | 404.62 | 404.70 | 404.83 | 404.87 | 0.04 | 0.96 | 3-6 |
| 57-13-6 | urea | $CO(NH_2)_2$ | O1s | 535.91 | 536.01 | 536.09 | 536.13 | 536.17 | 0.02 | 0.96 | 3-6 |
| 57-13-6 | urea | $CO(NH_2)_2$ | N1s | 405.40 | 405.58 | 405.67 | 405.79 | 405.84 | 0.04 | 0.97 | 3-6 |
| 57-13-6 | urea | $CO(NH_2)_2$ | C1s | 294.51 | 294.83 | 294.91 | 295.07 | 295.16 | 0.04 | 0.97 | 3-6 |
| 74-89-5 | methylamine | $CH_3NH_2$ | N1s | 404.51 | 404.55 | 404.67 | 404.79 | 404.90 | 0.06 | 0.95 | 4,5,6 |
| 98-95-3 | nitrobenzene | $C_6H_5NO_2$ | O1s | 537.64 | 537.70 | 537.77 | 537.83 | 537.84 | 0.03 | 0.91 | 3-6 |
| 98-95-3 | nitrobenzene | $C_6H_5NO_2$ | N1s | 411.70 | 411.87 | 411.95 | 412.09 | 412.12 | 0.05 | 0.94 | 3-6 |
| 98-95-3 | nitrobenzene | $C_6H_5NO_2$ | C1s (C1) | 291.84 | 292.01 | 292.12 | 292.26 | 292.30 | 0.05 | 0.94 | 3-6 |
| 98-95-3 | nitrobenzene | $C_6H_5NO_2$ | C1s (C2-4) | 290.74 | 290.90 | 291.00 | 291.13 | 291.17 | 0.04 | 0.95 | 3-6 |
| 71-43-2 | benzene | $C_6H_6$ | C1s | 289.89 | 290.09 | 290.16 | 290.31 | 290.35 | 0.05 | 0.95 | 3-6 |
| 536-74-3 | phenylacetylene | $C_8H_6$ | C1s (C3) | 290.68 | 290.88 | 290.96 | 291.10 | 291.15 | 0.05 | 0.95 | 3-6 |
| 536-74-3 | phenylacetylene | $C_8H_6$ | C1s (C2) | 290.17 | 290.34 | 290.45 | 290.58 | 290.62 | 0.05 | 0.95 | 3-6 |
| 536-74-3 | phenylacetylene | $C_8H_6$ | C1s (C4-6) | 290.00 | 290.17 | 290.28 | 290.40 | 290.45 | 0.04 | 0.96 | 3-6 |
| 536-74-3 | phenylacetylene | $C_8H_6$ | C1s (C1) | 289.61 | 289.75 | 289.77 | 289.93 | 289.99 | 0.05 | 0.97 | 3,4,6 |

# References


(1) Myrseth, V.; Bozek, J. D.; Kukk, E.; Sæthre, L. J.; Thomas, T. D. Adiabatic and vertical carbon 1s ionization energies in representative small molecules. *J. Electron Spectrosc. Relat. Phenom.* **2002**, *122*, 57–63.

(2) Siegbahn, K.; Nordling, C.; Johansson, G.; Hedman, J.; Hedén, P. F.; Hamrin, K.; Gelius, U.; Bergmark, T.; Werme, L. O.; Manne, R.; Baer, Y. *ESCA applied to free molecules*; North-Holland Publishing Company Amsterdam-London, 1969; pp 119–126.

(3) Thomas, T. D.; Shaw, R. W. Accurate core ionization potentials and photoelectron kinetic energies for light elements. *J. Electron Spectrosc. Relat. Phenom.* **1974**, *5*, 1081–1094.

(4) Siegbahn, K.; Nordling, C.; Johansson, G.; Hedman, J.; Hedén, P. F.; Hamrin, K.; Gelius, U.; Bergmark, T.; Werme, L. O.; Manne, R.; Baer, Y. *ESCA applied to free molecules*; North-Holland Publishing Company Amsterdam-London, 1969; p 89.

(5) Thomas, T. D. X-ray photoelectron spectroscopy of halomethanes. *J. Am. Chem. Soc.* **1970**, *92*, 4184–4189.

(6) Bakke, A. A.; Chen, H.-W.; Jolly, W. L. A table of absolute core-electron binding-energies for gaseous atoms and molecules. *J. Electron Spectrosc. Relat. Phenom.* **1980**, *20*, 333–366.

(7) Mills, B. E.; Martin, R. L.; Shirley, D. A. Further studies of the core binding energy-proton affinity correlation in molecules. *J. Am. Chem. Soc.* **1976**, *98*, 2380–2385.

(8) Siegbahn, K.; Nordling, C.; Johansson, G.; Hedman, J.; Hedén, P. F.; Hamrin, K.; Gelius, U.; Bergmark, T.; Werme, L. O.; Manne, R.; Baer, Y. *ESCA applied to free molecules*; North-Holland Publishing Company Amsterdam-London, 1969; pp 11–12.

(9) Drake, J. E.; Riddle, C.; Henderson, H. E.; Glavinčevski, B. ESCA investigations of Group IV derivatives. Part III. Binding energies for methyl substituted disilyl and digermyl chalcogenide series. *Can. J. Chem.* **1977**, *55*, 2957–2961.

(10) Naves de Brito, A.; Correia, N.; Svensson, S.; Ågren, H. A theoretical study of x-ray photoelectron spectra of model molecules for polymethylmethacrylate. *J. Chem. Phys.* **1991**, *95*, 2965–2974.

(11) Mocellin, A.; Wiesner, K.; Sorensen, S. L.; Miron, C.; Le Guen, K.; Céolin, D.; Simon, M.; Morin, P.; Bueno Machado, A.; Björneholm, O.; Naves de Brito, A. Site selective dissociation upon core ionization of ozone. *Chem. Phys. Lett.* **2007**, *435*, 214–218.

(12) Finn, P.; Pearson, R. K.; Hollander, J. M.; Jolly, W. L. Chemical shifts in core electron binding energies for some gaseous nitrogen compounds. *Inorg. Chem.* **1971**, *10*, 378–381.

(13) Naves de Brito, A.; Svensson, S.; Ågren, H.; Delhalle, J. Experimental and theoretical study of the XPS core levels of gas phase acetonitrile, acrylonitrile and propionitrile. Model molecules for polyacrylonitrile. *J. Electron Spectrosc. Relat. Phenom.* **1993**, *63*, 239–251.

(14) Plekan, O.; Feyer, V.; Richter, R.; Coreno, M.; de Simone, M.; Prince, K. C.; Carravetta, V. Investigation of the Amino Acids Glycine, Proline, and Methionine by Photoemission Spectroscopy. *J. Phys. Chem. A* **2007**, *111*, 10998–11005.

(15) Cavell, R. G.; Allison, D. A. Site of protonation in aromatic and acyclic amines and acyclic amides revealed by N1s core level electron spectroscopy. *J. Am. Chem. Soc.* **1977**, *99*, 4203–4204.

(16) Myrseth, V.; Børve, K. J.; Thomas, T. D. The Substituent Effect of the Methyl Group. Carbon 1s Ionization Energies, Proton Affinities, and Reactivities of the Methylbenzenes. *J. Org. Chem.* **2007**, *72*, 5715–5723.

(17) Carravetta, V.; Iucci, G.; Ferri, A.; Russo, M. V.; Stranges, S.; de Simone, M.; Polzonetti, G. Synchrotron radiation photoemission study of some $\pi$-conjugated alkynes in the gas phase: Experiment and theory. *Chem. Phys.* **2001**, *264*, 175 – 186.
